# Supplementary material for: Mitigating Selection Bias with Node Pruning and Auxiliary Options
Source: arXiv:2409.18857 source file (2025-05-17)
Supplement: Supplementary file 1 [file ethics.tex]

\section{Broader Impact}
This work reveals and mitigates a type of bias present in recent large language models~(LLMs).
Considering that LLMs have become an integral part in various applications from customer service to science, the presence of any type of bias can negatively impact reliability of systems and degrade precision in model- or data-driven decision making.
By addressing the bias, our research not only improves the accuracy and fairness of these models but also has potential in enhancing trustworthiness of LLMs in general.
Moreover, this work serves as a foundation for ongoing efforts to scrutinize and enhance LLM-automated systems, introducing a new perspective of analyzing performance.
